# Supplementary material for: Mechanochemical Morphodynamics of Active Bacterial Cells
Source: arXiv:2409.12681 source file (2024-09-24)
Supplement: Supplementary file 1 [file Supplementary_Information.pdf]

# Mechanochemical Morphodynamics of Active Bacterial Cells

Joydip Chaudhuri*
*Department of Chemical Engineering, Indian Institute of Technology Kharagpur, Kharagpur 721302, West Bengal, India*

## SUPPLEMENTARY INFORMATION

### A. Growth dynamics

The temporal equations in the manuscript (Equations (7) and (12)) depict the dynamics governing the evolution of the radius for spherical and cylindrical cells, respectively, as illustrated in Figures S1 and S2.

According to equation (13) of the manuscript, the temporal evolution of cell length ($L_C$) is indicated to be linear with respect to time ($t$), as the right-hand side of equation (13) remains independent of $L_C$. Figure S3 indicates this linear temporal evolution of cell length ($L_C$) in case of cylindrical cells. The length and time scales of the dynamics of these shape parameters vary significantly compared to the previous studies in the literature and matches quite well with the experimental results [1–4] and previous theories [5, 6].

### B. Linear stability analysis (LSA)

We conduct LSA on the steady-state equations (5) to (13) of the main manuscript, introducing perturbations in both the steady-state cell radii ($R_S$ and $R_C$) along the axial direction $z$ for both spherical and cylindrical cells.

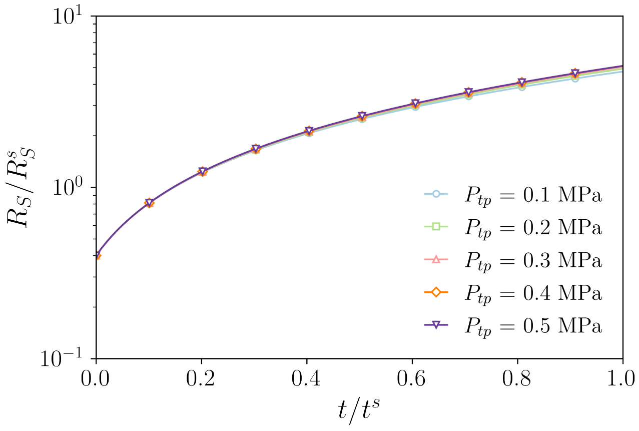


FIG. S1. Dynamics of radius ($R_S$) of cylindrical cell normalized by the steady-state radius ($R_S^s$) with time ($t$) normalized by the time to reach the steady-state radius ($t^s$) for different turgor pressures ($P_{tp}$).

* joy@che.iitkgp.ac.in

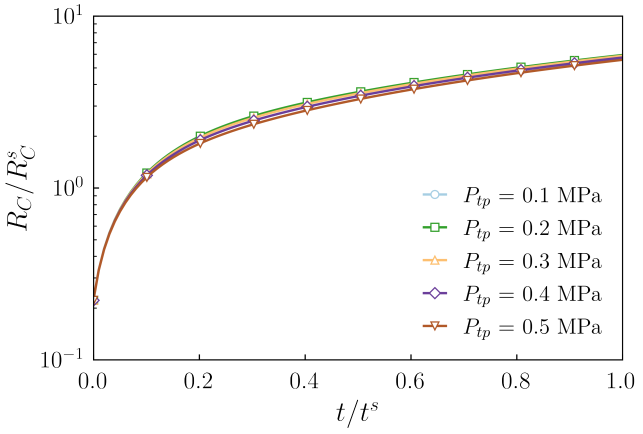


FIG. S2. Dynamics of radius ($R_C$) of cylindrical cell normalized by the steady-state radius ($R_C^s$) with time ($t$) normalized by the time to reach the steady-state radius($t^s$) for different turgor pressures ($P_{tp}$).

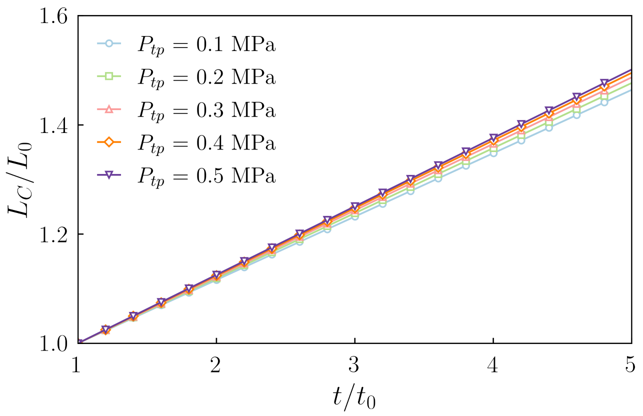


FIG. S3. Dynamics of length ($L_C$) of cylindrical cell normalized by the initial value ($L_0$) with time ($t$) normalized by the initial time ($t_0$) for different turgor pressures ($P_{tp}$).

The perturbations take the following forms:

$$R_S = R_S^s(z,t) + \widetilde{R}_S(t)e^{\omega t + ikz}, \tag{1}$$

$$R_C = R_C^s(z,t) + \widetilde{R}_C(t)e^{\omega t + ikz}, \tag{2}$$

where, $\omega$ is the complex growth rate, $k$ ($> 0$) is the wave number, and $\widetilde{R}_S(t) \ll R_S^s(z,t)$, $\widetilde{R}_C(t) \ll R_C^s(z,t)$, are the amplitudes of the perturbations and $i = \sqrt{-1}$.

The dispersion relation for the spherical cells with elas-

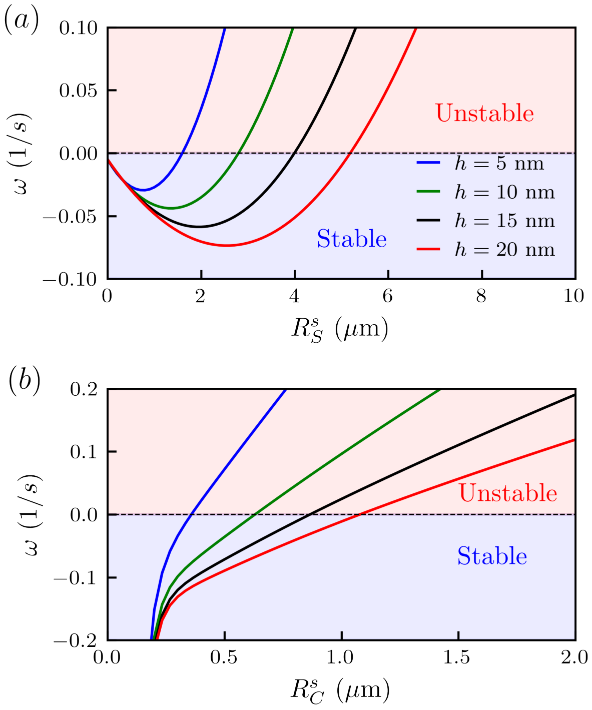


FIG. S4. Variation of the growth rate of the perturbation ($\omega$) with steady state radius of ($a$) spherical cells ($R_S^s$) and ($b$) cylindrical cells ($R_C^s$) for different cell wall thicknesses ($h$).

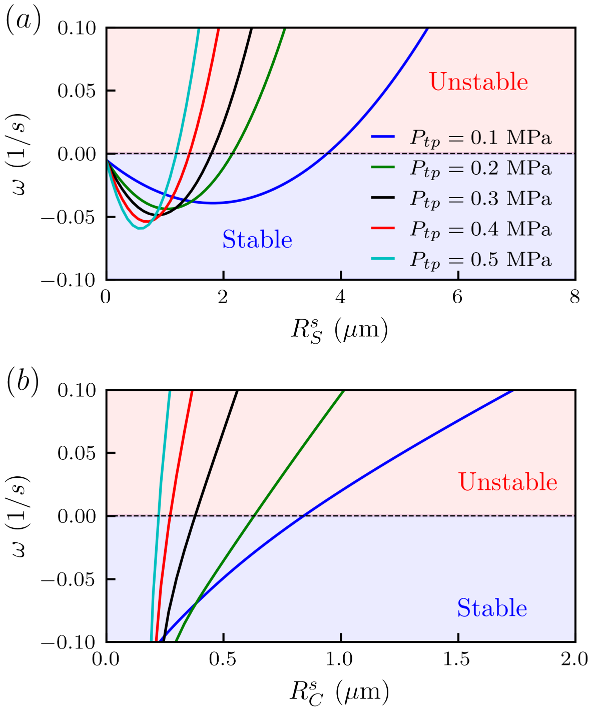


FIG. S5. Variation of the growth rate of the perturbation ($\omega$) with steady state radius of ($a$) spherical cells ($R_S^s$) and ($b$) cylindrical cells ($R_C^s$) for different turgor pressures ($P_{tp}$).

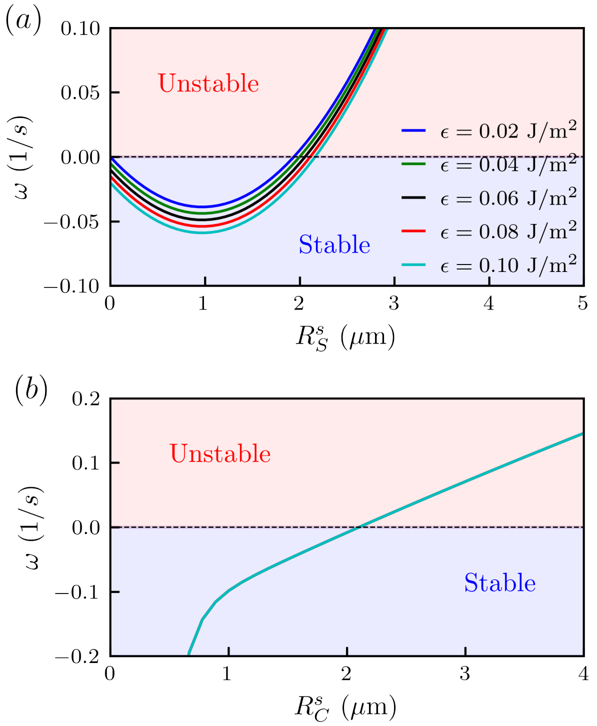


FIG. S6. Variation of the growth rate of the perturbation ($\omega$) with steady state radius of ($a$) spherical cells ($R_S^s$) and ($b$) cylindrical cells ($R_C^s$) for different energy released ($\epsilon$).

tic cell walls obtained from the LSA can be written as,

$$\omega = 4\pi Q_R^S \left[ -12 P_S \left(R_S^s\right)^2 + \left( \frac{P_{tp}^2}{2\sigma_0} + 2P_{tp} \right) R_S^s + 2\epsilon - 2\sigma \right]. \quad (3)$$

The steady state radius ($R_S^s$) for spherical cells from LSA is obtained from neutral stability points which are evaluated from Equation 3 by enforcing $\omega = 0$.

For the simplified case of spherical cells with plastic cell walls where $\sigma$ is constant, equation 3 reduces to,

$$\omega = 4\pi Q_R^S \left[ -12 P_S \left(R_S^s\right)^2 + 2P_{tp} R_S^s + 2\left(\epsilon - \sigma\right) \right]. \quad (4)$$

The dispersion relation for the cylindrical cells obtained from the LSA can be expressed as,

$$\omega = -2\pi Q_R^C L_C \left[ 6P_C R_C^s - P_{tp} + \frac{k}{\left(R_C^s\right)^2} \left( \frac{1}{R_0} - \frac{2}{R_C^s} \right) - \frac{k}{R_C^s} \left( \frac{1}{R_0} - \frac{1}{\left(R_C^s\right)^2} \right) \right]. \quad (5)$$

Again, the steady state radius ($R_C^s$) for cylindrical cells from LSA is obtained from neutral stability points which are evaluated from Equation 5 by enforcing $\omega = 0$.

We employed LSA to assess $R^s$ for both spherical ($R_S^s$) and cylindrical ($R_C^s$) bacterial cells across various crucial

thermodynamic parameters, specifically $h, P_{tp}$, and $\epsilon$, as depicted in Figures S4 − S6. The plots in figures S4 − S6 show the variation of the growth rate of the perturbation ($\omega$) with the variation of the radius of the ($a$) spherical ($R^s_S$) (with elastic cell walls) and ($b$) cylindrical cells ($R^s_C$) for different $h, P_{tp}$, and $\epsilon$, respectively. A perturbation is unstable when $\omega > 0$ such that wave-like bulges nucleate on the cell-wall with growing amplitude, whereas, it is stable when $\omega < 0$ such that any wave-like bulges will essentially die down with time and the cell will retain its shape. Neutral stability curves are evaluated from $\omega = 0$, which concurrently yields a set of steady-state radii ($R^s$) evaluated through LSA.


[1] J. J. Thwaites and N. H. Mendelson, Adv. Microb. Physiol. **32**, 173 (1991).

[2] M. T. Cabeen, G. Charbon, W. Vollmer, P. Born, N. Ausmees, D. B. Weibel, and C. Jacobs-Wagner, The EMBO journal **28**, 1208 (2009).

[3] S. Takeuchi, W. R. DiLuzio, D. B. Weibel, and G. M. Whitesides, Nano letters **5**, 1819 (2005).

[4] K. D. Young, Microbiol. Mol. Biol. Rev. **70**, 660 (2006).

[5] H. Jiang and S. X. Sun, Phys. Rev. Lett. **105**, 028101 (2010).

[6] S. Banerjee, N. F. Scherer, and A. R. Dinner, Soft Matter **12**, 3442 (2016).
